# Supplementary material for: Small Space Stream Summary for Matroid Center
Source: arXiv:1810.06267 source file (2020-07-20)
Supplement: Supplementary file 1 [file appendix.tex]

\section{Appendix}
\label{sec:appendix}
%\subsection{Proofs of Missing Lemmas}
%\input{matroid_inter}
\input{offline}

%%% Local Variables:
%%% mode: latex
%%% TeX-master: "matroid_center"
%%% End:
